# Supplementary material for: The Bayesian Infinitesimal Jackknife for Variance
Source: arXiv:2305.06466 source file (2024-06-26)
Supplement: Supplementary file 1 [file appendix_high_dim_residual.tex]

\def\postlthat{\p(\lambda | \ftdist, N, \gammahat)}

\def\lambdatil{\tilde{\lambda}}
\def\gltil{\gamma, \lambdatil}
\def\glltil{\gamma, \lambda, \lambdatil}

\def\ellcorrg#1#2#3{\sigma^{#1}_{#2}\left(#3\right)}
\def\ellcorr#1#2{\sigma_{#1}\left(#2\right)}

\def\postltil{\p(\lambdatil \vert \ftdist, N, \gammahat)}

\def\mugrad#1{\mu_{(#1)}}
\def\mubar#1#2{\bar{\mu}_{(#1)}\left(#2\right)}

\def\cetwohat{\underline{\hat{\overline{\mathcal{K}}}}^{\ell\ell}}

\def\sumh{\sum_{h=1}^{G}}

%%%%%%%%%%%%%%%%%%%%%%%%%%%%%%%%%%%%%%%%%%%%%%%%%%%%%%%%%%%%%%%%%%%%%%%%
%%%%%%%%%%%%%%%%%%%%%%%%%%%%%%%%%%%%%%%%%%%%%%%%%%%%%%%%%%%%%%%%%%%%%%%%
%%%%%%%%%%%%%%%%%%%%%%%%%%%%%%%%%%%%%%%%%%%%%%%%%%%%%%%%%%%%%%%%%%%%%%%%

Recall that
% Let us suppress the $\t$ dependence for the moment and write

\begin{align*}
\resid{T}(\t) ={}&
\frac{1}{N^2}  \sum_{n=1}^N\sum_{m=1}^N \htil(x_n, x_m)
\nonumber \textrm{ where } \\
\htil(\x_n, \x_m) ={}&
N^2 \expect{\postgt}{
    \gbar(\gamma) \cetwo(\x_n, \x_m \vert \gamma)
    }.
\end{align*}

Following \lemref{centered_expectations}, and 
letting $\gammahat = \gammahat(\t)$ (suppressing
the $\t$ dependence for brevity), define the centered quantities

\begin{align*}
\varepsilon_g :={}& \g(\gammahat) - \expect{\postgt}{\g(\gamma)} \\
\varepsilon_K(\x_n, \x_m) :={}&
    \cetwo(\x_n, \x_m \vert \gammahat) -
    \expect{\postgt}{\cetwo(\x_n, \x_m \vert \gamma)}\\
\ghat(\gamma) :={}& \g(\gamma) - \g(\gammahat) \\
\cetwohat(\x_n, \x_m \vert \gamma) :={}&
    \cetwo(\x_n, \x_m \vert \gamma) - \cetwo(\x_n, \x_m \vert \gammahat).
\end{align*}

Apply \thmref{bayes_clt_main} repeatedly to give
\begin{align*}
\varepsilon_g ={}& 
    \ordp{N^{-1}} \ggrad{1}(\gammahat) +
    \ordp{N^{-1}} \ggrad{2}(\gammahat) +
    \ordlog{N^{-2}} \resid{g} \\
\varepsilon_K(\x_n, \x_m) ={}&
    \ordp{N^{-1}} \cetwograd{1}(\x_n, \x_m \vert \gammahat) +
    \ordp{N^{-1}} \cetwograd{2}(\x_n, \x_m \vert \gammahat) +
    \ordlog{N^{-2}} \resid{K} \\
\expect{\postgt}{\ghat(\gamma) \cetwohat(\x_n, \x_m \vert \gamma)} ={}&
    \ordp{N^{-1}}
        \ggrad{1}(\gammahat) \cetwograd{1}(\x_n, \x_m \vert \gammahat) +
    \ordlog{N^{-2}} \resid{gK}(\x_n, \x_m),
\end{align*}
where in the late term we have applied \thmref{bayes_clt_main} with the index
set $\indexset = [N]\times[N]$ (see \defref{bclt_okay_index} in
\secref{index_sets}).

Then we can use \lemref{centered_expectations} to give
\begin{align*}
\MoveEqLeft
\htil(\x_n, \x_m) 
={}\\\MoveEqLeft
N^2 \expect{\postgt}{\gbar(\gamma) \cetwo(\x_n, \x_m \vert \gamma)}
={}\\\MoveEqLeft
    N^2 \left( 
        \expect{\postgt}{\ghat(\gamma) \cetwohat(\x_n, \x_m \vert \gamma)} -
        \varepsilon_g \varepsilon_K(\x_n, \x_m) \right)
={}\\\MoveEqLeft
N^2 \left(
    \ordp{N^{-1}}
    \ggrad{1}(\gammahat) \cetwograd{1}(\x_n, \x_m \vert \gammahat) +
\ordlog{N^{-2}} \resid{gK}(\x_n, \x_m)
\right) -
\\&
N^2 \left(
    \ordp{N^{-1}} \ggrad{1}(\gammahat) +
    \ordp{N^{-1}} \ggrad{2}(\gammahat) +
    \ordlog{N^{-2}} \resid{g}
    \right) \times
\\&\quad\quad\left(
    \ordp{N^{-1}} \cetwograd{1}(\x_n, \x_m \vert \gammahat) +
    \ordp{N^{-1}} \cetwograd{2}(\x_n, \x_m \vert \gammahat) +
    \ordlog{N^{-2}} \resid{K}
    \right)
={}\\\MoveEqLeft
\ordp{N}
    \ggrad{1}(\gammahat) \cetwograd{1}(\x_n, \x_m \vert \gammahat) - 
\\&
\ordlog{1}\Big(
    \left(\ggrad{1}(\gammahat) + \ggrad{2}(\gammahat)\right) 
        \cetwograd{2}(\x_n, \x_m \vert \gammahat) +
    \ggrad{2}(\gammahat) \cetwograd{1}(\x_n, \x_m \vert \gammahat) -
    \resid{gK}(\x_n, \x_m)
\Big)  +
\\& \ordlogp{N^{-1}},
\end{align*}
where the $\ordlogp{N^{-3}}$ term goes to zero even when
summed over $n,m$.

Defining
\begin{align*}
    V_1 :={}& \meannm \cetwograd{1}(\x_n, \x_m \vert \gammahat) \\
    V_2 :={}& \meannm \cetwograd{2}(\x_n, \x_m \vert \gammahat),
\end{align*}
it follows that
\begin{align*}
\sqrt{N} \resid{T}(\t) ={}&
\ordp{N^{3/2}} V_1 + \ordlogp{N^{1/2}}\left(V_1 + V_2\right) + 
    \ordlogp{N^{-1/2}},
\end{align*}
so it suffices to show that $N^{3/2} V_1 \rightarrow \infty$
and $V_1 = \ordlogp{V_2}$.

Recall that
\begin{align*}
%
% \ceone(\x_n \vert \gamma) :={}& \expect{\postl}{\ellbarbar(\x_n \vert \gl)} \\
\cetwo(\x_n, \x_m \vert \gammahat) :={}&
    \expect{\postlthat}{
        \ellbarbar(\x_n \vert \gammahat, \lambda)
        \ellbarbar(\x_m \vert \gammahat, \lambda)
    }.
\end{align*}
By interchanging differentiation and integration and recalling
that the posterior is fixed in the expectation, we have
\begin{align*}
    \expect{\fdist(\x_n) \fdist(\x_m)}{\cetwograd{1}(\x_n, \x_m \vert \gammahat)} = 0
    \quad\textrm{and}\quad
    \expect{\fdist(\x_n) \fdist(\x_m)}{\cetwograd{2}(\x_n, \x_m \vert \gammahat)} = 0.
\end{align*}

Therefore, to apply an asymptotic theory of V-statistics (\lemref{ustat}) to
$V_1$, we need to compute
\begin{align*}
\var{\fdistnm}{\cetwograd{1}(\x_n, \x_m \vert \gammahat)} =
    \expect{\fdistnm}{\cetwograd{1}(\x_n, \x_m \vert \gammahat)^2}.
\end{align*}

We can differentiate as in \appref{post_derivs} to get
\begin{align}
\MoveEqLeft
\cetwograd{1}(\x_n, \x_m \vert \gammahat) ={} \nonumber\\&
\expect{\postlthat}{
    \ellbarbargrad{1}(\x_n \vert \gammahat, \lambda)
    \ellbarbar(\x_m \vert \gammahat, \lambda) +
    \ellbarbar(\x_n \vert \gammahat, \lambda)
    \ellbarbargrad{1}(\x_m \vert \gammahat, \lambda) +
    \ellbarbar(\x_n \vert \gammahat, \lambda)
    \ellbarbar(\x_m \vert \gammahat, \lambda)
    \ellgrad{1}(\lambda \vert \gammahat, \xvec)
    \eqlabel{cetwogradoneexpansion}
}.
% \expect{\p(\lambda | \ftdist, N, \gammahat)}{
%     \ellbarbargrad{1}(\x_n \vert \gammahat, \lambda)
%     \ellbarbar(\x_m \vert \gammahat, \lambda)
%     } +
% {}
% \expect{\p(\lambda | \ftdist, N, \gammahat)}{
%     \ellbarbar(\x_n \vert \gammahat, \lambda)
%     \ellbarbargrad{1}(\x_m \vert \gammahat, \lambda)
%     } +
% \\{}&
% \expect{\p(\lambda | \ftdist, N, \gammahat)}{
%     \ellbarbar(\x_n \vert \gammahat, \lambda)
%     \ellbarbar(\x_m \vert \gammahat, \lambda)
%     \ellgrad{1}(\lambda \vert \gammahat, \xvec)
%     },
%
\end{align}

\def\funder{\underline{f}}
Consder a generic quantity of the form 
$\expect{\postlthat}{\funder_1(\x_n, \lambda) \funder_2(\x_m, \lambda)}$,
where $\expect{\fdist(\x_n)}{\funder_1(\x_n)} = 0$ and $\expect{\fdist(\x_m)}{\funder_2(\x_m)} = 0$.
By Fubini's theorem,
\begin{align}
\MoveEqLeft
\expect{\fdistnm}{\expect{\postlthat}{\funder_1(\x_n, \lambda) \funder_2(\x_m, \lambda)}^2}
=\nonumber\\{}&
\expect{\fdistnm}{
    \int \funder_1(\x_n, \lambda) \funder_2(\x_m, \lambda) \postlthat d\lambda
    \int \funder_1(\x_n, \lambdatil) \funder_2(\x_m, \lambdatil) \postltil d\lambdatil
}
=\\{}&
\int \int
    \expect{\fdist(\x_n)}{\funder_1(\x_n, \lambda) \funder_1(\x_n, \lambdatil)}
    \expect{\fdist(\x_m)}{\funder_2(\x_m, \lambda) \funder_2(\x_m, \lambdatil)}
     \postlt \postltil  d\lambda d\lambdatil.
     \eqlabel{variance_of_expectation}
\end{align}
With this in mind, define
\begin{align*}
\ellcorr{jk}{\glltil} :={}&
\expect{\fdist(\xn)}{
    \ellbarbargrad{j}(\xn \vert \gl)
    \ellbarbargrad{k}(\xn \vert \gltil)
},
\end{align*}
where in a slight abuse of notation we take $\ellbarbargrad{0}(\x_n \vert \gl) =
\ellbarbar(\x_n \vert \gl)$.

In general, the quantity $\ellcorr{jk}{\gammahat,
\lambda, \lambdatil}$ does not vanish asymptotically, in the sense that there
will exist some set $A$, such that  $\int_A \ellcorr{jk}{\gammahat, \lambda,
\lambdatil} \p(\lambda \vert \xvec, \gammahat) \postlt \postltil
d\lambda d\lambdatil$ is bounded away from zero even as $N
\rightarrow \infty$, and combining
\eqref{cetwogradoneexpansion} and \eqref{variance_of_expectation}, we
see that
\begin{align*}
\MoveEqLeft
\expect{\fdistnm}{\cetwograd{1}(\x_n, \x_m \vert \gammahat)^2} =
\int \int \Big(
\\&\quad
\ellcorr{11}{\glltil} \ellcorr{00}{\glltil} +
\ellcorr{00}{\glltil} \ellcorr{11}{\glltil} +
\\&\quad
\ellcorr{00}{\glltil} \ellcorr{00}{\glltil}
\ellgrad{1}(\lambda \vert \gamma, \xvec)
\ellgrad{1}(\lambdatil \vert \gamma, \xvec) +
\\&\quad
\ellcorr{10}{\glltil} \ellcorr{01}{\glltil} +
\ellcorr{01}{\glltil} \ellcorr{10}{\glltil} +
\\&\quad
\ellcorr{10}{\glltil} \ellcorr{00}{\glltil}
\ellgrad{1}(\lambdatil \vert \gamma, \xvec) +
\ellcorr{10}{\glltil} \ellcorr{00}{\glltil}
\ellgrad{1}(\lambda \vert \gamma, \xvec) +
\\&\quad
\ellcorr{00}{\glltil} \ellcorr{10}{\glltil}
\ellgrad{1}(\lambdatil \vert \gamma, \xvec) +
\ellcorr{00}{\glltil} \ellcorr{10}{\glltil}
\ellgrad{1}(\lambda \vert \gamma, \xvec)
\Big)\\&
\postlt \postltil
d\lambda d\lambdatil  = \ord{1}.
\end{align*}

In general, we thus expect that $\var{\fdistnm}{\cetwograd{1}(\x_n, \x_m \vert
\gammahat)}$ to be $\ord{1}$ and nonzero in general.  An analogous argument
gives that $\var{\fdistnm}{\cetwograd{2}(\x_n, \x_m \vert \gammahat)} = \ord{1}$
as well.

From this and \lemref{ustat} it follows that $N V_1 = \ordp{1}$
and $N V_2 = \ordp{1}$.  Then $N^{3/2} V_1 \rightarrow \infty$,
and $\sqrt{N} \resid{T}(\t) \rightarrow \infty$ as well.

\begin{ex}

In particular, in the case of \exref{re}, we can define
\begin{align*}
\ellbar^g(\y_n \vert \gamma, \lambda_g) :={}&
    \ell(\y_n \vert \gamma, \lambda_g, \a_{ng} = 1) -
    \expect{\postglt}{\ell^g(\y_n \vert \gamma, \lambda_g, \a_{ng} = 1)}\\
\mu^g(\gamma, \lambda_g) :={}&
    \expect{\fdist(\y_n \vert \a_{ng} = 1)}
           {\ellbar^g(\y_n \vert \gamma, \lambda_g)}\\
\ellbarbar^g(\x_n \vert \gamma, \lambda_g) :={}&
   \a_{ng} \ellbar^g(\y_n \vert \gamma, \lambda_g) -
   \frac{1}{G} \mu^g(\gamma, \lambda_g)
   % \expect{\fdist(\y_n \vert \a_{ng} = 1)}
   %        {\ellbar^g(\y_n \vert \gamma, \lambda_g)}
%         \Rightarrow  \\
% \ellbar(\x_n \vert \gl) :={}&
%    \sumg \sumn \a_{ng} \ellbar^g(\y_n \vert \gamma, \lambda_g)\\
% \expect{\fdist(\xn)}{\ellbar(\xn \vert \gl)} ={}&
%     \sumg \expect{\fdist(\a_{0g})}{\a_{0g}} \ellbar^g(\gamma, \lambda_g)
% =   \frac{1}{G} \sumg \ellbar^g(\gamma, \lambda_g) \\
%
\end{align*}
and also defining
\begin{align*}
\mu(\gl) := \frac{1}{G} \mu^g(\gamma, \lambda_g)
\end{align*}
so that
\begin{align*}
\ellbarbar(\x_n \vert \gl) :={}&
    \sumg \ellbarbar^g(\x_n \vert \gamma, \lambda_g)
\quad\textrm{where} \\
    \expect{\fdist(\xn)}{\ellbarbar^g(\xn \vert \gamma, \lambda_g)} ={}& 0
    \quad\textrm{and} \quad
    \expect{\postglt}{\ellbarbar^g(\xn \vert \gamma, \lambda_g)} ={} 0,
\end{align*}
and $\ellbarbar^g(\x_n \vert \gamma, \lambda_g)$ depends only on $\lambda_g$.

We can thus define
\begin{align*}
\ellcorrg{g}{ab}{\gamma, \lambda_g, \lambdatil_g} :={}&
    \expect{\fdist(\y_0 \vert \a_{ng} = 1)}{
        \ellbarbargrad{a}^{g}(\y_0 \vert \gamma, \lambda_g)
        \ellbarbargrad{b}^{g}(\y_0 \vert \gamma, \lambdatil_g)}
\\
\mubar{ab}{\glltil} :={}&
    \frac{1}{G^2} \sumg \sumh
        \mugrad{a}^g(\gamma, \lambda_g)
        \mugrad{b}^h(\gamma, \lambdatil_h)
\end{align*}
noting that
\begin{align*}
\MoveEqLeft
\expect{\fdist(\xn)}{
    \ellbarbargrad{a}(\xn \vert \gl)
    \ellbarbargrad{b}(\xn \vert \gltil)}
=\\{}&
\expect{\fdist(\xn)}{
    \sumg \ellbarbargrad{a}^g(\xn \vert \gl)
    \sumh \ellbarbargrad{b}^h(\xn \vert \gltil)}
=\\{}&
\expect{\fdist(\xn)}{
    \sumg \left(
        \a_{ng} \ellbargrad{a}^g(\y_n \vert \gamma, \lambda_g) -
        \frac{1}{G} \mugrad{a}^g(\gamma, \lambda_g)
    \right)
    \sumh \left(
        \a_{nh} \ellbargrad{b}^h(\y_n \vert \gamma, \lambdatil_h) -
        \frac{1}{G} \mugrad{b}^h(\gamma, \lambdatil_h)
    \right)
}
=\\{}& \frac{1}{G} \sumg \ellcorrg{g}{ab}{\gamma, \lambda_g, \lambdatil_g}
    - \mubar{ab}{\glltil}.
\end{align*}
Since we expect $\ellcorrg{g}{ab}{\gamma, \lambda_g, \lambdatil_g}$ to
be a non-degenerate random variable, we expect $\sqrt{N}\resid{t}$ not to
vanish in \exref{re}, no matter how large $G$ and $N$ are.

\end{ex}
