# Supplementary material for: The Bayesian Infinitesimal Jackknife for Variance
Source: arXiv:2305.06466 source file (2024-06-26)
Supplement: Supplementary file 2 [file delta_method_standard_errors.tex]

In order to evaluate our results we need to estimate standard errors for each of
these quantities.  Note that, even in the absence of MCMC error (e.g. as $M
\rightarrow \infty$), we would not expect $\gcovijhat = \gcovboothat$, as the two
numerically distinct despite being consistent estimates of the same quantity.
Similarly, under correct specification, we do not expect $\gcovijhat = \gcovboothat =
\gcovbayes$ even when there is no MCMC error.  Thus, when comparing our
estimated $\gcovijhat$, $\gcovboothat$, and $\gcovbayeshat$, it is important to
consider sampling error due to the randomness in the original sample $\xvec$ in
addition to MCMC error.

To do so, we rely on two algorithms to estimate the frequentist and MCMC
variability of scalar covaraince estimates.  We will apply these two algorithms
to the components of $\gcovijhat$ and $\gcovboothat$, neglecting sampling
covariance between elements of the matrices.  Of course, the elements of
the covaraince matrices are not independent, and so the standard errors we
compute are useful heuristics but should not be used for formal hypothesis
testing.

Our first algorithm uses the classical delta method for the sampling covariance
of a sample covariance of IID draws.

%%%%%%%%%%%%%%%%%%%%%%%%%%%%%%%%%%%%%
%%%%%%%%%%%%%%%%%%%%%%%%%%%%%%%%%%%%%

\begin{algorithm}[H]
\caption{Delta Method for IID Data}\algrlabel{deltamethodalg}
\textbf{Inputs (global variables):}\\
$a = (a_1, \ldots, a_N)$ \Comment{Scalar IID draws}\\
$b = (b_1, \ldots, b_N)$ \Comment{Scalar IID draws}\\
\begin{algorithmic}
%\algrlabel{Compute Sampling covariance of}
%
\Function{SampleCov}{$\alpha$, $\beta$}
\State \Return
    $\meann \alpha_n \beta_n - \meann \alpha_n \meann \beta_n$
\EndFunction\\
%
%\Call{SampleCov}{$a$, $b$}
\Function{SampleCovDeltaMethodSE}{$a$, $b$}
    \State $\bar{a} \gets \meann a_n$
    \State $\bar{b} \gets \meann b_n$
    \State $\bar{ab} \gets \meann a_n b_n$
    \State $ab \gets \meann a \odot b$
    \Comment{The $\odot$ operator denotes the element-wise product}
    \State $\nabla h \gets \left(1, -\bar{a}, -\bar{b}\right)$
    \State $S \gets
    \left[
    \begin{matrix}
    \Call{SampleCov}{ab, ab} &
    \Call{SampleCov}{ab, a} &
    \Call{SampleCov}{ab, b} \\
    \Call{SampleCov}{a, ab} &
    \Call{SampleCov}{a, a} &
    \Call{SampleCov}{a, b} \\
    \Call{SampleCov}{b, ab} &
    \Call{SampleCov}{b, a} &
    \Call{SampleCov}{b, b} \\
    \end{matrix}
    \right]$
    \State \Return $\sqrt{\frac{1}{N} \nabla h^T S \nabla h}$
\EndFunction\\
\end{algorithmic}
\end{algorithm}

%%%%%%%%%%%%%%%%%%%%%%%%%%%%%%%%%%%%%
%%%%%%%%%%%%%%%%%%%%%%%%%%%%%%%%%%%%%

The bootstrap draws of the posterior mean, $\gamma^*_b$, are IID given the
original dataset, $\xvec$, since the MCMC chains and bootstrap samples are
independent across $b$. The variability in the draws $\gamma^*_b$ reflect both
MCMC and sampling variability, since both the MCMC chains and bootstrap draws
are different for each.  Consequently, we can estimate both the frequentist and
MCMC variability in $\gcovboothat$ by applying \algrref{deltamethodalg} to each
pair of components of $\gamma^*_b$.  Let $\gamma^*_{i\cdot}$ denote the
length-$B$ vector of the $i$-the element of the posterior means, and let
$\seboot$ be the $\gdim\times\gdim$ matrix whose $i,j$-th element is
\begin{align*}
\seboot_{ij} :=
    \Call{SampleCovDeltaMethodSE}{\gamma^*_{i\cdot}, \gamma^*_{j\cdot}}.
\end{align*}
We can thus approximately expect that
$\gcovboothat_{ij} \in \left(\gcovtrue_{ij} \pm 2 \seboot_{ij} \right)$.

Similarly, we can treat the $\infl_n$ of \algrref{ijalg} as IID draws from
$\fdist(\x_n)$, and use \algrref{deltamethodalg} to estimate the frequentist
sampling error of the $i,j$-the component $\gcovij_{ij}$.  Specifically,
letting $\infl_{i\cdot}$ denote the length-$N$ vector containing the $i$-th
component of the influence score, we define
\begin{align*}
\seijfreq_{ij} :=
    \Call{SampleCovDeltaMethodSE}{\infl_{i\cdot}, \infl_{j\cdot}}.
\end{align*}
We can thus approximately expect that
$\gcovij_{ij} \in \left(\gcovtrue_{ij} \pm 2 \seijfreq_{ij} \right)$.

However, we cannot use \algrref{deltamethodalg} to capture the difference
between $\gcovij$ and $\gcovijhat$.  To do so, we block bootstrap the MCMC chain
with a block size much larger than the estimated effective sample size,
applying \algrref{ijalg} to each resampled chain, computing an estimated
MCMC standard error, $\seijmcmc$.  Finally, we combine the two sources of
error assuming independence, giving, for each $i,j$,
\begin{align*}
\seij_{ij} := \sqrt{(\seijmcmc_{ij})^2 + (\seijfreq_{ij})^2}.
\end{align*}
We can thus approximately expect that
$\gcovijhat_{ij} \in \left(\gcovtrue_{ij} \pm 2 \seij_{ij} \right)$.

% Note that
% multivariate autoregressive techniques such as \cite{flegal:2020:mcmcse}
% will be difficult to employ...
